# Supplementary material for: A similarity renormalization group approach to Green's function methods
Source: arXiv:2303.05984 source file (2023-05-17)
Supplement: Supplementary file 1 [file si.pdf]

# Supporting Information for "A similarity renormalization group approach to Green's function methods"

Antoine Marie[1, a)] and Pierre-François Loos[1, b)]
*Laboratoire de Chimie et Physique Quantiques (UMR 5626), Université de Toulouse, CNRS, UPS, France*

## S1. SRG-$G_0W_0$, ev$GW$ and SRG-ev$GW$ statistics

In this section, the values obtained with the two alternative SRG-based methods derived in the main manuscript, SRG-$G_0W_0$ and SRG-ev$GW$, are reported along with their corresponding histogram plot of the errors. For the sake of completeness, the SRG-regularized self-energy and quasiparticle equation used for the SRG-$G_0W_0$ and SRG-ev$GW$ calculations are reported below:

$$\epsilon_p^{\text{HF}} + \Sigma_{pp}^{\text{SRG-}GW}(\omega) - \omega = 0, \tag{S1}$$

with

$$\Sigma_{pp}^{\text{SRG-}GW}(\omega) = \sum_{i\nu} \frac{(W_{pi}^{\nu})^2}{\omega - \epsilon_i + \Omega_\nu} e^{-2(\epsilon_p - \epsilon_i + \Omega_\nu)^2 s} + \sum_{a\nu} \frac{(W_{pa}^{\nu})^2}{\omega - \epsilon_a - \Omega_\nu} e^{-2(\epsilon_p - \epsilon_a - \Omega_\nu)^2 s}, \tag{S2}$$

Therefore, the SRG-$G_0W_0$ values are obtained by solving once these equations (one-shot procedure) without linearization, while the SRG-ev$GW$ results correspond to solutions of these equations where self-consistency on the $\epsilon_p$'s has been reached.

One observe in Table S1 that the $G_0W_0$ and SRG-$G_0W_0$ values are the same for all systems (up to $10^{-2}$eV). Figure S2 shows that ev$GW$ provides a slight improvement over $G_0W_0$, while ev$GW$ and SRG-ev$GW$ perform similarly. One interesting fact is that the convergence of SRG-ev$GW$ deteriorates faster than for SRG-qs$GW$ with respect to $s$. We suspect that it is due to the absence of the off-diagonal terms.

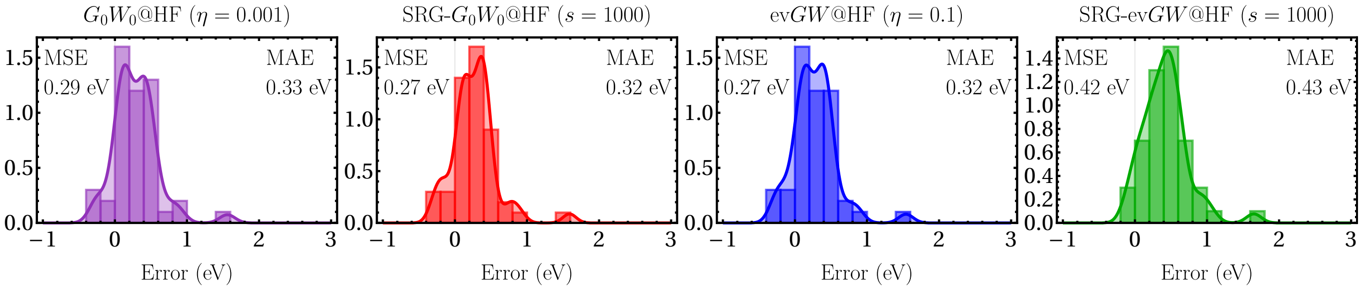


FIG. S1. Histogram of the errors [with respect to ΔCCSD(T)] for the principal IP of the $GW$50 test set calculated using $G_0W_0$@HF, SRG-$G_0W_0$@HF, ev$GW$, and SRG-ev$GW$. All calculations are performed with the aug-cc-pVTZ basis.

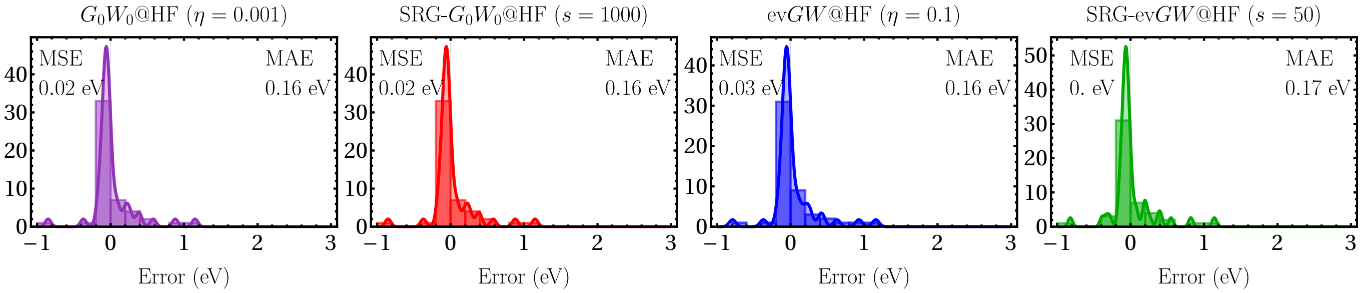


FIG. S2. Histogram of the errors [with respect to ΔCCSD(T)] for the principal EA of the $GW$50 test set calculated using $G_0W_0$@HF, SRG-$G_0W_0$@HF, ev$GW$, and SRG-ev$GW$. All calculations are performed with the aug-cc-pVTZ basis.

a)Electronic mail: amarie@irsamc.ups-tlse.fr
b)Electronic mail: loos@irsamc.ups-tlse.fr

TABLE S1. Principal IP and EA (in eV) of the $GW50$ test set calculated using ΔCCSD(T) (reference), $G_0W_0$@HF, SRG-$G_0W_0$@HF, ev$GW$, and SRG-ev$GW$. The statistical descriptors associated with the errors with respect to the reference values are also reported. All calculations are performed with the aug-cc-pVTZ basis.

| | Principal IP | | | | | Principal EA | | | | |
|---|---|---|---|---|---|---|---|---|---|---|
| Mol. | ΔCCSD(T) (Ref.) | $G_0W_0$@HF ($\eta = 10^{-3}$) | SRG-$G_0W_0$@HF ($s = 10^3$) | ev$GW$ ($\eta = 10^{-1}$) | SRG-ev$GW$ ($s = 50$) | ΔCCSD(T) (Ref.) | $G_0W_0$@HF ($\eta = 10^{-3}$) | SRG-$G_0W_0$@HF ($s = 10^3$) | ev$GW$ ($\eta = 10^{-1}$) | SRG-ev$GW$ ($s = 50$) |
| He | 24.54 | 24.59 | 24.59 | 24.58 | 24.57 | −2.66 | −2.66 | −2.66 | −2.66 | −2.66 |
| Ne | 21.47 | 21.46 | 21.46 | 21.30 | 21.29 | −5.09 | −5.25 | −5.25 | −5.24 | −5.24 |
| $H_2$ | 16.40 | 16.49 | 16.49 | 16.52 | 16.51 | −1.35 | −1.28 | −1.28 | −1.28 | −1.28 |
| $Li_2$ | 5.25 | 5.38 | 5.38 | 5.44 | 5.42 | 0.34 | 0.17 | 0.17 | 0.16 | 0.17 |
| LiH | 8.02 | 8.22 | 8.22 | 8.26 | 8.23 | −0.29 | 0.27 | 0.27 | 0.27 | 0.27 |
| HF | 16.15 | 16.25 | 16.25 | 16.10 | 16.09 | −0.66 | −0.71 | −0.71 | −0.71 | −0.71 |
| Ar | 15.60 | 15.72 | 15.72 | 15.67 | 15.66 | −2.55 | −2.68 | −2.68 | −2.67 | −2.67 |
| $H_2O$ | 12.69 | 12.90 | 12.90 | 12.80 | 12.79 | −0.61 | −0.68 | −0.68 | −0.68 | −0.68 |
| LiF | 11.47 | 11.40 | 11.40 | 11.20 | 11.18 | 0.35 | 0.33 | 0.33 | 0.33 | 0.33 |
| HCl | 12.67 | 12.78 | 12.78 | 12.76 | 12.75 | −0.57 | −0.64 | −0.64 | −0.64 | −0.64 |
| BeO | 9.95 | 9.74 | 9.74 | 9.64 | 9.61 | 2.17 | 2.28 | 2.28 | 2.30 | 2.31 |
| CO | 13.99 | 14.80 | 14.80 | 14.77 | 14.76 | −1.57 | −1.66 | −1.66 | −1.65 | −1.65 |
| $N_2$ | 15.54 | 17.10 | 17.10 | 17.10 | 17.09 | −2.37 | −2.10 | −2.10 | −2.10 | −2.10 |
| $CH_4$ | 14.39 | 14.76 | 14.76 | 14.76 | 14.75 | −0.65 | −0.70 | −0.70 | −0.69 | −0.69 |
| $BH_3$ | 13.31 | 13.68 | 13.68 | 13.70 | 13.69 | −0.09 | −0.46 | −0.46 | −0.46 | −0.45 |
| $NH_3$ | 10.91 | 11.22 | 11.22 | 11.19 | 11.17 | −0.61 | −0.68 | −0.68 | −0.68 | −0.68 |
| BF | 11.15 | 11.34 | 11.34 | 11.37 | 11.36 | −0.80 | −0.90 | −0.90 | −0.90 | −0.90 |
| BN | 12.05 | 11.76 | 11.76 | 11.78 | 11.76 | 3.02 | 3.90 | 3.90 | 3.95 | 3.95 |
| $SH_2$ | 10.39 | 10.51 | 10.51 | 10.51 | 10.50 | −0.52 | −0.60 | −0.60 | −0.60 | −0.60 |
| $F_2$ | 15.81 | 16.35 | 16.35 | 16.15 | 16.14 | 0.32 | −0.53 | −0.53 | −0.47 | −0.47 |
| MgO | 7.97 | 8.40 | 8.40 | 8.34 | 8.28 | 1.54 | 1.64 | 1.64 | 1.65 | 1.66 |
| $O_3$ | 12.85 | 13.56 | 13.56 | 13.53 | 13.51 | 1.82 | 2.19 | 2.19 | 2.25 | 2.25 |
| $C_2H_2$ | 11.45 | 11.57 | 11.57 | 11.60 | 11.59 | −0.80 | −0.71 | −0.71 | −0.71 | −0.71 |
| HCN | 13.76 | 13.86 | 13.86 | 13.87 | 13.86 | −0.53 | −0.52 | −0.52 | −0.52 | −0.52 |
| $B_2H_6$ | 12.27 | 12.81 | 12.81 | 12.81 | 12.80 | −0.52 | −0.56 | −0.56 | −0.56 | −0.56 |
| $CH_2O$ | 10.93 | 11.39 | 11.39 | 11.34 | 11.32 | −0.60 | −0.61 | −0.61 | −0.60 | −0.60 |
| $C_2H_4$ | 10.69 | 10.74 | 10.74 | 10.78 | 10.77 | −1.90 | −0.75 | −0.75 | −0.74 | −0.74 |
| $SiH_4$ | 12.79 | 13.22 | 13.22 | 13.23 | 13.22 | −0.53 | −0.59 | −0.59 | −0.59 | −0.59 |
| $PH_3$ | 10.60 | 10.79 | 10.79 | 10.82 | 10.81 | −0.51 | −0.58 | −0.58 | −0.58 | −0.58 |
| $CH_4O$ | 11.09 | 11.55 | 11.55 | 11.48 | 11.47 | −0.59 | −0.64 | −0.64 | −0.64 | −0.64 |
| $H_2NNH_2$ | 9.49 | 9.84 | 9.84 | 9.80 | 9.79 | −0.60 | −0.69 | −0.69 | −0.68 | −0.68 |
| HOOH | 11.51 | 11.96 | 11.96 | 11.85 | 11.83 | −0.96 | −0.75 | −0.75 | −0.75 | −0.75 |
| KH | 6.32 | 6.44 | 6.44 | 6.48 | 6.42 | 0.30 | 0.28 | 0.28 | 0.28 | 0.28 |
| $Na_2$ | 4.93 | 4.98 | 4.98 | 5.03 | 5.02 | 0.36 | 0.26 | 0.26 | 0.24 | 0.26 |
| $HN_3$ | 10.77 | 11.12 | 11.12 | 11.11 | 11.10 | −0.51 | −0.6 | −0.6 | −0.59 | −0.59 |
| $CO_2$ | 13.80 | 14.24 | 14.24 | 14.16 | 14.15 | −0.88 | −0.98 | −0.98 | −0.97 | −0.97 |
| PN | 11.90 | 12.33 | 12.33 | 12.34 | 12.33 | −0.02 | −0.03 | −0.03 | 0.01 | 0.01 |
| $CH_2O_2$ | 11.54 | 12.00 | 12.00 | 11.90 | 11.88 | −0.63 | −0.69 | −0.69 | −0.68 | −0.68 |
| $C_4$ | 11.43 | 11.77 | 11.77 | 11.77 | 11.76 | 2.38 | 2.24 | 2.24 | 2.34 | 2.35 |
| $C_3H_6$ | 10.83 | 11.20 | 11.20 | 11.20 | 11.19 | −0.94 | −0.75 | −0.75 | −0.75 | −0.75 |
| $C_2H_3F$ | 10.63 | 10.84 | 10.84 | 10.85 | 10.84 | −0.65 | −0.69 | −0.69 | −0.68 | −0.68 |
| $C_2H_4O$ | 10.29 | 10.84 | 10.84 | 10.76 | 10.75 | −0.54 | −0.56 | −0.56 | −0.56 | −0.56 |
| $C_2H_6O$ | 10.82 | 11.37 | 11.37 | 11.31 | 11.30 | −0.58 | −0.65 | −0.65 | −0.64 | −0.64 |
| $C_3H_8$ | 12.13 | 12.61 | 12.61 | 12.60 | 12.59 | −0.63 | −0.70 | −0.70 | −0.70 | −0.70 |
| NaCl | 9.10 | 9.20 | 9.20 | 9.16 | 9.13 | 0.67 | 0.64 | 0.64 | 0.64 | 0.64 |
| $P_2$ | 10.72 | 10.49 | 10.49 | 10.52 | 10.51 | 0.43 | 0.47 | 0.47 | 0.53 | 0.54 |
| $MgF_2$ | 13.93 | 13.94 | 13.94 | 13.74 | 13.72 | 0.29 | 0.15 | 0.15 | 0.16 | 0.16 |
| OCS | 11.23 | 11.52 | 11.52 | 11.50 | 11.49 | −1.43 | −1.03 | −1.03 | −1.02 | −1.01 |
| $SO_2$ | 10.48 | 11.38 | 11.38 | 11.34 | 11.33 | 2.24 | 2.82 | 2.82 | 2.87 | 2.88 |
| $C_2H_3Cl$ | 10.17 | 10.39 | 10.39 | 10.39 | 10.38 | −0.61 | −0.66 | −0.66 | −0.65 | −0.65 |
| MSE | | 0.29 | 0.29 | 0.26 | 0.25 | | 0.02 | 0.02 | 0.03 | 0.00 |
| MAE | | 0.33 | 0.33 | 0.32 | 0.31 | | 0.16 | 0.16 | 0.16 | 0.17 |
| RMSE | | 0.43 | 0.43 | 0.41 | 0.40 | | 0.28 | 0.28 | 0.29 | 0.28 |
| SDE | | 0.31 | 0.31 | 0.31 | 0.32 | | 0.29 | 0.29 | 0.29 | 0.29 |
| Min | | −0.29 | −0.29 | −0.31 | −0.34 | | −0.85 | −0.85 | −0.79 | −0.82 |
| Max | | 1.56 | 1.56 | 1.56 | 1.55 | | 1.15 | 1.15 | 1.16 | 1.14 |
